# Supplementary material for: Determination of effective mechanical properties of a double-layer beam by means of a nano-electromechanical transducer
Source: arXiv:1407.6867 source file (2014-07-25)
Supplement: Supplementary file 1 [file Hocke_Duffing_arXiv_Supplemental_Material.pdf]

# Supplemental Material: Determination of effective mechanical properties of a double-layer beam by means of a nano-electromechanical transducer

Fredrik Hocke,[1,2,3] Matthias Pernpeintner,[1,2,3] Xiaoqing Zhou,[4] Albert Schliesser,[4,5] Tobias J. Kippenberg,[4] Hans Huebl,[1,2,a)] and Rudolf Gross[1,2,3,b)]

[1)] *Walther-Meißner-Institut, D-85748 Garching, Germany*

[2)] *Nanosystems Initiative Munich, D-80799 München, Germany*

[3)] *Technische Universität München, D-85748 Garching, Germany*

[4)] *École Polytechnique Fédérale de Lausanne, CH-1015 Lausanne, Switzerland*

[5)] *Niels Bohr Institute, University of Copenhagen, DK-2100 Copenhagen, Denmark*

(Dated: 24 July 2014)

[a)] hans.huebl@wmi.badw.de

[b)] Rudolf.Gross@wmi.badw.de

## A. MECHANICS OF A NANOBEAM WITH HOMOGENEOUS CROSS-SECTION

### a. Equation of motion

We consider a volume element of the beam with length $dx$ as indicated in Fig. S1. The cross-sectional area of the beam is denoted $A$. The beam is aligned along the $x$-axis, the displacement $v(x)$ is in $y$-direction (we restrict our discussion to the transverse vibration). According to standard beam theory[S1], the bending of the beam is associated with a shear force $F_\mathrm{s}(x)$ and a torque $M(x)$ (along the $z$-direction) acting on the infinitesimal volume element depicted in Fig. S1. The net force in $y$-direction applied to the volume element is then given by $dF_\mathrm{bending} = -\frac{\partial F_\mathrm{s}}{\partial x}dx$. Here, the minus sign is due to sign convention of Ref.[S2] illustrated in Fig. S1. The net moment on the volume element, $\frac{\partial M}{\partial x}dx$, is related to the shear force $F_\mathrm{s}$ by[S1,S2]

$$\frac{\partial M}{\partial x}dx = F_\mathrm{s}\frac{dx}{2} + \left(F_\mathrm{s} + \frac{\partial F_\mathrm{s}}{\partial x}dx\right)\frac{dx}{2} \approx F_\mathrm{s}dx. \tag{S1}$$

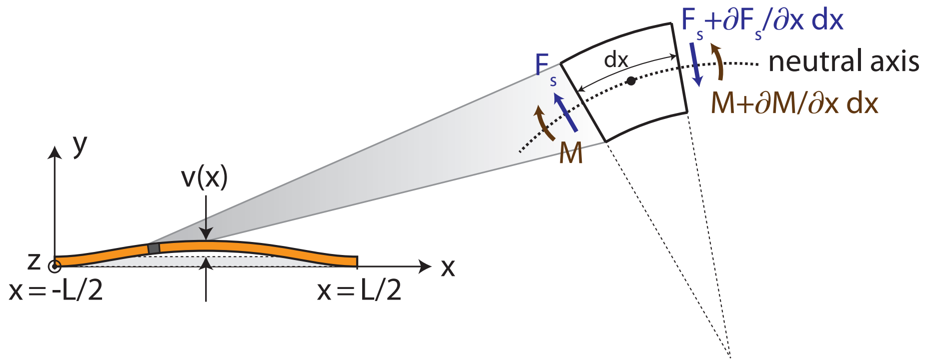


FIG. S1. Shear force and torque due to bending of the beam, following the beam sign convention in[S2].

For a prestressed beam, there are additional axial forces $F_\mathrm{ax,1}$ and $F_\mathrm{ax,2}$ acting on the volume element, as indicated in Fig. S2. They are given by

$$\mathbf{F}_\mathrm{ax,1} = \sigma_0 A(-\cos\varphi_1\hat{\mathbf{x}} + \sin\varphi_1\hat{\mathbf{y}})$$

$$\mathbf{F}_\mathrm{ax,2} = \sigma_0 A(\cos\varphi_2\hat{\mathbf{x}} - \sin\varphi_2\hat{\mathbf{y}}),$$

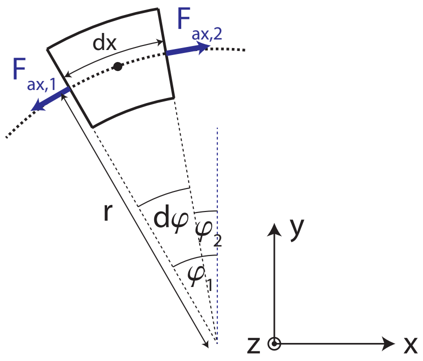


FIG. S2. Axial force in a prestressed beam.

where $\sigma_0$ is the prestress. The net force due to the prestress is then given by

$$d\mathbf{F}_{\text{prestress}} = \mathbf{F}_{\text{ax},2} + \mathbf{F}_{\text{ax},1} = \sigma_0 A \left[ (\cos\varphi_2 - \cos\varphi_1)\hat{\mathbf{x}} + (\sin\varphi_1 - \sin\varphi_2)\hat{\mathbf{y}} \right] \ .$$

For small displacement of the beam ($v \ll L$ and $\varphi_{1,2} \ll 1$), we can use the approximations $\cos\varphi_2 - \cos\varphi_1 \approx 0$ and $\sin\varphi_1 - \sin\varphi_2 \approx \varphi_1 - \varphi_2 = d\varphi$. Furthermore, we have $d\varphi \approx dx/r$ and the curvature radius $r$ is given by[S3]

$$\frac{1}{r} = \frac{\frac{\partial^2 v}{\partial x^2}}{\left[1 + \left(\frac{\partial v}{\partial x}\right)^2\right]^{3/2}} \approx \frac{\partial^2 v}{\partial x^2} \ .$$

For the approximation on the right-hand side we have have used $\partial v/\partial x \ll 1$ for small displacement. With the above approximations we finally get

$$d\mathbf{F}_{\text{prestress}} = \sigma_0 A dx \, \frac{\partial^2 v}{\partial x^2} \, \hat{\mathbf{y}}. \qquad \text{(S2)}$$

Note that the axial force due to the prestress does not contribute to the bending moment acting on the volume element.

The total force on the volume element, acting in $y$-direction, is the sum of the axial force due to prestress, $dF_{\text{prestress}}$, and the shear force due to bending, $dF_{\text{bending}} = -\frac{\partial F_{\text{s}}}{\partial x} dx$.

### b. Relation between bending moment and displacement curvature

As mentioned above, an axial force due to prestress does not cause any bending moment. Therefore, we can neglect the prestress in this subsection and assume $\sigma_0 = 0$.

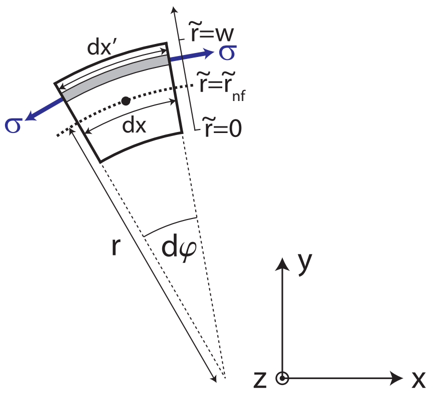


FIG. S3. Derivation of the relation between torque and curvature of the beam.

In order to derive the relation between the bending moment $M$ and the curvature of the beam $\partial^2 v/\partial x^2$, we consider the volume element shown in Fig. S3. By definition, the length of the neutral axis $\tilde{r} = \tilde{r}_{\mathrm{nf}}$ does not change under influence of a bending moment, while the other layers of the beam are elongated ($\tilde{r} > \tilde{r}_{\mathrm{nf}}$) resp. compressed ($\tilde{r} < \tilde{r}_{\mathrm{nf}}$). The change in length of such a layer is given by

$$dx' - dx = dx\frac{\tilde{r} - \tilde{r}_{\mathrm{nf}}}{r} \ .$$

This results in a stress[S3]

$$\sigma = E\,\frac{dx' - dx}{dx} = E\,\frac{\tilde{r} - \tilde{r}_{\mathrm{nf}}}{r} \tag{S3}$$

corresponding to the torque

$$dM = \sigma t d\tilde{r}(\tilde{r} - \tilde{r}_{\mathrm{nf}}) = Etd\tilde{r}\,\frac{(\tilde{r} - \tilde{r}_{\mathrm{nf}})^2}{r} \ . \tag{S4}$$

Here, $t$ denotes the thickness of the beam (along the $z$-axis).

The total bending moment can be calculated by integration of $dM$:

$$M = \int_{\tilde{r}=0}^{w} dM = \int_{\tilde{r}=0}^{w} Etd\tilde{r}\frac{(\tilde{r} - \tilde{r}_{\mathrm{nf}})^2}{r} \ ,$$

where $w$ is the width of the beam. In case of a homogeneous beam, the neutral axis is in the center of the beam, $\tilde{r}_{\mathrm{nf}} = w/2$, and we get $M = Ew^3t/(12r)$. Defining the area moment of inertia as $I = w^3t/12$ and using $1/r \approx \partial^2 v/\partial x^2$ yields[S3,S4]

$$M = EI\frac{\partial^2 v}{\partial x^2} \ . \tag{S5}$$

With Eq. (S1) and $dF_{\mathrm{bending}} = -\frac{\partial F_s}{\partial x} dx$, we then obtain the relation

$$dF_{\mathrm{bending}} = -\frac{\partial^2 M}{\partial x^2} dx = -EI \frac{\partial^4 v}{\partial x^4} dx \;. \tag{S6}$$

## c. Equation of Motion and Resonance frequency of the beam

Using Eqs. (S2) and (S6), the total restoring force acting on the infinitesimal volume element can be expressed as

$$dF_{\mathrm{restoring}} = dF_{\mathrm{bending}} + dF_{\mathrm{prestress}} = -EI \frac{\partial^4 v}{\partial x^4} dx + \sigma_0 A dx \frac{\partial^2 v}{\partial x^2} \;. \tag{S7}$$

This results in the equation of motion for the transverse vibrational mode of the beam[S1,S5]

$$-EI \frac{\partial^4 v}{\partial x^4} + \sigma_0 A \frac{\partial^2 v}{\partial x^2} = \rho A \frac{\partial^2 v}{\partial t^2} \;, \tag{S8}$$

where $\rho$ denotes the mass density of the volume element.

To solve this equation of motion, we first assume a harmonic time-dependence $v(x,t) = v(x)\exp(-i\omega t)$, which leads to the following differential equation for $v(x)$[S1]:

$$-EI \frac{\partial^4 v(x)}{\partial x^4} + \sigma_0 A \frac{\partial^2 v(x)}{\partial x^2} = -\rho A \omega^2 v(x) \;. \tag{S9}$$

The general solution of this differential equation is

$$v(x) = c_1 \exp(\alpha x) + c_2 \exp(-\alpha x) + c_3 \sin(\beta x) + c_4 \cos(\beta x) \tag{S10}$$

with

$$\begin{aligned} \mu_{\pm} &= \frac{\sigma_0 A \pm \sqrt{\sigma_0^2 A^2 + 4EI\rho A \omega^2}}{2EI} \\ I &= \frac{w^3 t}{12} \\ \alpha &= \sqrt{\mu_+} > 0 \\ \beta &= -\imath\sqrt{\mu_-} > 0 \;. \end{aligned}$$

For a doubly-clamped beam, the boundary conditions are[S1,S4]

$$\begin{aligned} v(x = -L/2) &= 0 \\ v(x = L/2) &= 0 \\ \frac{\partial v(x = -L/2)}{\partial x} &= 0 \\ \frac{\partial v(x = +L/2)}{\partial x} &= 0 \;. \end{aligned} \tag{S11}$$

The application of these boundary conditions to the general solution (S10) results in a homogeneous linear system of four equations and four variables $c_i$ ($i = 1, 2, 3, 4$). The determinant of this system of equations has to vanish, which is a necessary condition for the existence of solutions. As the determinant is a function of $\omega$, this allows to determine the resonance frequency $\omega/2\pi$ of the beam.

The determinant can be written down analytically. However, it is highly non-linear in $\omega$ with no known analytical solutions. Therefore, we employ numerical methods to determine the resonance frequency.

### d. Comparison to the approximative formula for prestressed beams

According to Verbridge *et al.*[S6], the resonance frequency of a prestressed nanomechanical beam is given by

$$\omega_i = \frac{i^2\pi^2}{L^2}\sqrt{\frac{EI}{\rho A}}\sqrt{1+\frac{\sigma_0 A L^2}{i^2 E I \pi^2}}\,, \tag{S12}$$

where $i = 1$ for the fundamental vibrational mode. This expression, however, is exact only for simply supported beams and therefore does not accurately reproduce the resonance frequency of a doubly-clamped beam. The latter can numerically be determined by finding the zeros of the determinant of the boundary matrix coefficients as described above. However, it is not possible to provide an analytical expression. In the following, we will compare the numerically determined resonance frequency of the experimentally studied nanobeam with the value given by Eq. (S12).

## B. DOUBLE-LAYER BEAMS

Up to now, we have focused on a beam with homogeneous cross-section. Here, we extend our discussion to beams consisting of two layers stacked in $z$-direction with thickness $t_\mathrm{A}$ and $t_\mathrm{B}$, as illustrated in Fig. S4. The Young's modulus and prestress of the two layers are denoted $E_\mathrm{A}$ and $E_\mathrm{B}$ resp. $\sigma_{0,\mathrm{A}}$ and $\sigma_{0,\mathrm{B}}$. This scheme is rather generic and thus can be extended to more than two layers. As we restrict the discussion to the in-plane motion of the beam, the displacement $v(x)$ is along $\hat{\mathbf{y}}$.

Again, we consider an infinitesimal volume element of the nanobeam as illustrated in Fig. S4. The restoring forces $dF_\mathrm{re,A}$ and $dF_\mathrm{re,B}$ arising from bending and elongation of the

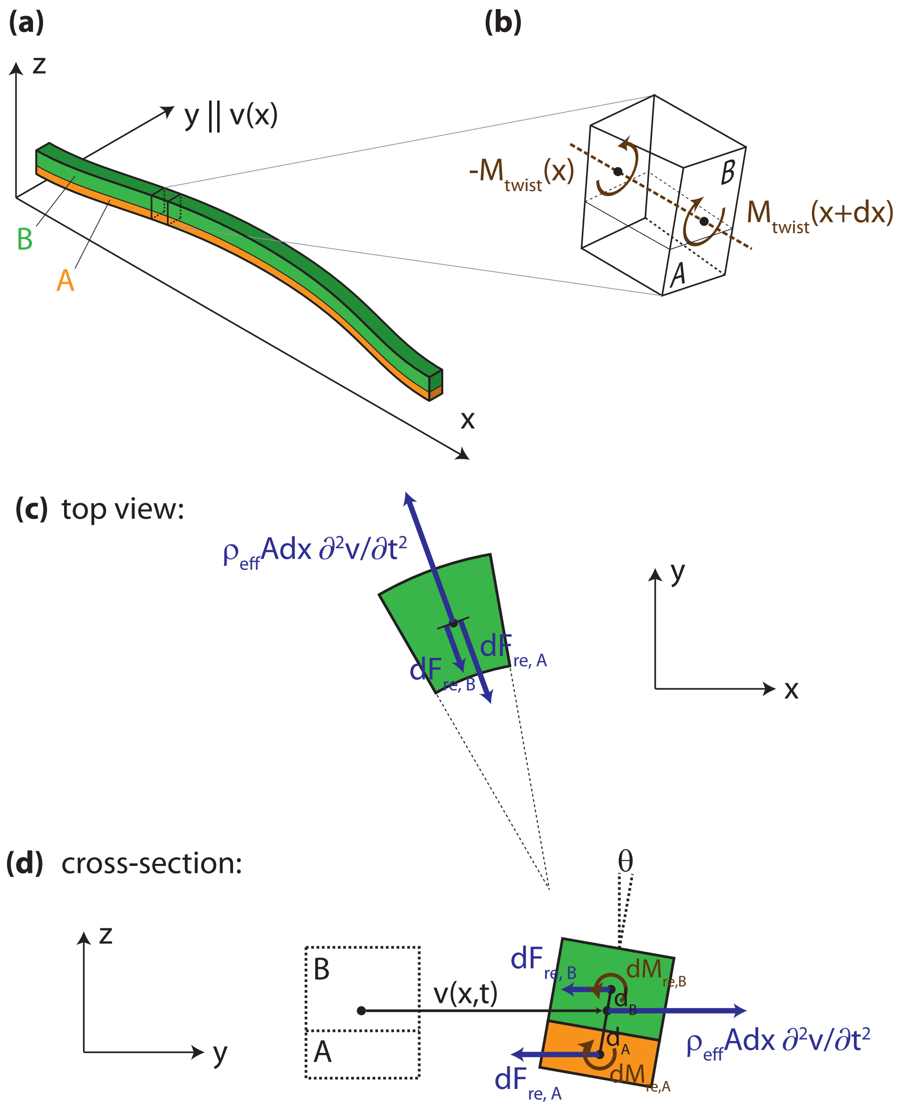


FIG. S4. **a.** Schematic illustration of the in-plane vibrational motion of the double-layer nanomechanical beam. **b.** Infinitesimal volume element of the beam with dimensions $dx \times b \times (t_{\mathrm{A}} + t_{\mathrm{B}})$. Tilt and torsion of the volume element are indicated. **c** and **d.** Top view and cross-sectional view of the volume element, illustrating the restoring forces and corresponding torques.

two beam layers A and B act on the respective centers of mass of the two layers A and B of the volume element. The distance between the center of mass of A (B) and the center of mass of the whole volume element is denoted $d_{\mathrm{A}}$ $(d_{\mathrm{B}})$. As the restoring forces $dF_{\mathrm{re},i}$ $(i = \mathrm{A}, \mathrm{B})$ do not act on the center of mass of the volume element, they induce a torque $dM_{\mathrm{re},i} = dF_{\mathrm{re},i} d_i$ along $\hat{\mathbf{x}}$ on the volume element as depicted in Fig. S4(d). The net torque

is then given by $dM_{\mathrm{re}} = dM_{\mathrm{re,A}} - dM_{\mathrm{re,B}}$. This torque induces a tilt (angle $\theta$) of the volume element so that the in-plane vibrational mode is accompanied by an oscillating $x$-dependent torsion of the double-layer beam.

In the following, we will show that the corresponding tilt angles $\theta(x)$ are small and the torsional energy is about four orders of magnitude smaller than the total energy stored in the beam vibration. Therefore, the contribution of the beam torsion may be neglected when describing the in-plane motion of the double-layer nanobeam, as shown in more detail in Sec. B d.

### a. Vibrational in-plane motion

We first focus of the vibrational motion of the double-layer beam neglecting beam torsion. We show that the vibrational motion of a double-layer beam can be described analogous to the homogeneous beam by defining effective material parameters. Later on, we also turn to the torsional degree of freedom and estimate the tilt angle $\theta$ of the torsional motion as well as the corresponding energy stored in the torsion of the beam. With that, we show that the torsional motion can indeed be neglected.

For a double-layer beam, the restoring force acting on the infinitesimal volume element is given by [see Fig. S4(c)]

$$dF_{\mathrm{re}} = dF_{\mathrm{re,A}} + dF_{\mathrm{re,B}} \ ,$$

where $dF_{\mathrm{re},i} = dF_{\mathrm{prestress},i} + dF_{\mathrm{bending},i}$ ($i = \mathrm{A}, \mathrm{B}$) as defined in Eq. (S7). With the effective density $\rho_{\mathrm{eff}} = (\rho_{\mathrm{A}} t_{\mathrm{A}} + \rho_{\mathrm{B}} t_{\mathrm{B}})/(t_{\mathrm{A}} + t_{\mathrm{B}})$ and the beam cross-sectional area $A = (t_{\mathrm{A}} + t_{\mathrm{B}})w$, Newton's second law for the volume element reads

$$dF_{\mathrm{re,A}} + dF_{\mathrm{re,B}} = \rho_{\mathrm{eff}} dx A \frac{\partial^2 v}{\partial t^2} \ .$$

Using Eqs. (S2) and (S6) and defining the effective Young's modulus

$$E_{\mathrm{eff}} = \frac{E_{\mathrm{A}} I_{\mathrm{A}} + E_{\mathrm{B}} I_{\mathrm{B}}}{I_{\mathrm{A}} + I_B} = \frac{E_{\mathrm{A}} t_{\mathrm{A}} + E_{\mathrm{B}} t_{\mathrm{B}}}{t_{\mathrm{A}} + t_{\mathrm{B}}}$$

and the effective prestress

$$\sigma_{\mathrm{eff}} = \frac{\sigma_{0,\mathrm{A}} t_{\mathrm{A}} + \sigma_{0,\mathrm{B}} t_{\mathrm{B}}}{t_{\mathrm{A}} + t_{\mathrm{B}}}$$

the resulting equation of motion for the double-layer beam reads

$$-E_{\mathrm{eff}} I \frac{\partial^4 v}{\partial x^4} + \sigma_{\mathrm{eff}} A \frac{\partial^2 v}{\partial x^2} = \rho_{\mathrm{eff}} A \frac{\partial^2 v}{\partial t^2} \ , \qquad \text{(S13)}$$

where $I = I_\mathrm{A} + I_\mathrm{B}$.

Equation (S13) is fully equivalent to Eq. (S8) if one replaces the material parameters $\rho$, $\sigma$ and $E$ by the effective material parameters $\rho_\mathrm{eff}$, $\sigma_\mathrm{eff}$ and $E_\mathrm{eff}$. Hence, the resonance frequency of a double-layer nanomechanical beam can – analogously to a homogeneous beam – be approximated by using Eq. (S12) or calculated numerically by solving Eq. (S9) with Eqs. (S10) and (S11) using effective parameters.

### b. Application to the presented sample

The nanomechanical beam discussed in the main text consists of a $t_\mathrm{A} = 70\,\mathrm{nm}$ thin, highly tensile-stressed silicon nitride layer, on which a $t_\mathrm{B} = 130\,\mathrm{nm}$ thick, compressively stressed niobium film has been deposited. Using $E_\mathrm{SiN} = 160\,\mathrm{GPa}$, $\sigma_{0,\mathrm{SiN}} = 830\,\mathrm{MPa}$ (both experimentally determined for a similar sample[S7]), $E_\mathrm{Nb} = 105\,\mathrm{GPa}$[S4], an estimated compressive stress in the Nb film of $\sigma_{0,\mathrm{Nb}} \approx -150\,\mathrm{MPa}$[S8], $\rho_\mathrm{SiN} = 3000\,\mathrm{kg/m^3}$[S9] and $\rho_\mathrm{Nb} = 8570\,\mathrm{kg/m^3}$[S4], we get

$$E_\mathrm{eff} = 124 \text{ GPa}$$
$$\sigma_\mathrm{eff} = 193 \text{ MPa}$$
$$\rho_\mathrm{eff} = 6621 \text{ kg/m}^3$$

Verbrigde's formula Eq. (S12) (without the right-hand side approximation) yields

$$\Omega_\mathrm{m} = 2\pi \times 1.42 \text{ MHz} ,$$

where we have used $L = 60\,\mu\mathrm{m}$ and $w = 140\,\mathrm{nm}$. For comparison, the numerical solution of the above described determinant leads to $\Omega_\mathrm{m} = 2\pi \times 1.48\,\mathrm{MHz}$, which deviates from the approximate expression (S12) by about 4%.

The numerical solution of Eqs. (S9), (S10) and (S11) also allows to calculate the shape of the fundamental vibrational mode, considering axial prestress and doubly-clamped boundary conditions. Figure S5 shows the resulting displacement of the beam $v(x)$ as a function of $x$, together with the $x$-dependent displacement of a doubly-clamped unstressed beam (cf.[S4]) and a simply-supported prestressed beam ($v(x) \approx v_0 \cos(\pi x/L)$, cf.[S1]).

Our calculation confirms that the displacement of the highly prestressed nanomechanical beam studied in our experiments can well be approximated by a cosine function as it is the

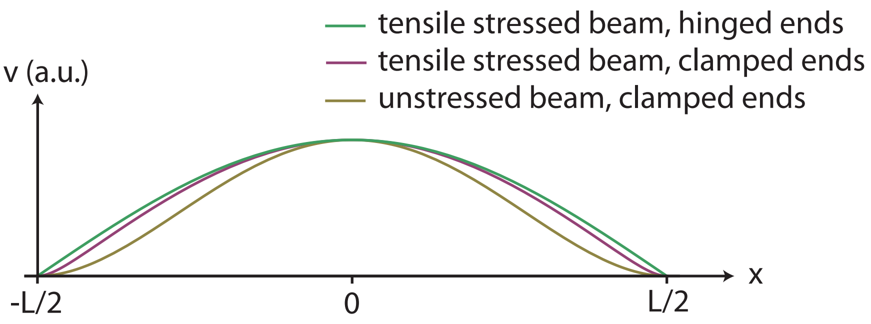


FIG. S5. Position dependent displacement of the tensile-stressed, doubly clamped beam compared to typical approximations.

case for a simply-supported prestressed beam. In the following estimation, we will therefore use this approximation instead of the more complex numerical solution.

### c. Torsional motion of the beam

Equation (S13), which describes the in-plane vibrational motion of a double-layer nanobeam, only holds for small beam torsion $\theta \ll 1$, where the displacement of the two beam layers from the equilibrium position is approximately equal: $v_{\mathrm{A}} \approx v_{\mathrm{B}} = v$. In the following, we will estimate the tilt angle $\theta$ of the in-plane beam motion and in this way justify the above assumption.

As illustrated in Figs. S4(b) and (d), there are two different types of torque acting on the volume element: First, we have $dM_{\mathrm{re}} = dM_{\mathrm{re,A}} - dM_{\mathrm{re,B}}$ (introduced at the beginning of Sec. B), which arises from the fact that the forces $dF_{\mathrm{re,A}}$ and $dF_{\mathrm{re,B}}$ act on the center of mass of the layers A and B and in general do not compensate each other:

$$dM_{\mathrm{re}} = dM_{\mathrm{re,A}} - dM_{\mathrm{re,B}} = dF_{\mathrm{re,A}} d_{\mathrm{A}} - dF_{\mathrm{re,B}} d_{\mathrm{B}} \; . \tag{S14}$$

Second, if the beam is twisted, there is a corresponding torque proportional to $\partial\theta/\partial x$ acting on the cross-section of the beam at $x$ and $x + dx$. This torque is – similar to $d\mathbf{M}_{\mathrm{re}}$ – directed along $\hat{\mathbf{x}}$ and is given by[S4]

$$M_{\mathrm{twist}}(x) = \mu I_{\mathrm{p}} \frac{\partial\theta(x)}{\partial x} \; , \tag{S15}$$

where $I_{\mathrm{p}}$ is the polar moment of inertia and $\mu$ the shear modulus. Summing up all torques along $\hat{\mathbf{x}}$ acting on the infinitesimal volume element leads to the equation of motion for the

torsion of the beam (compare[S4])

$$M_{\text{twist}}(x+dx) - M_{\text{twist}}(x) + dM_{\text{re}} = \rho I_{\text{p}} dx \, \frac{\partial^2 \theta}{\partial t^2} \ .$$

We use Eq. (S15) and expand $M_{\text{twist}}(x)$ in a Taylor series around $x$. Together with Eq. (S14), we then get

$$\mu I_{\text{p}} \frac{\partial^2 \theta}{\partial x^2} + \frac{dM_{\text{re}}}{dx} = \rho I_{\text{p}} \frac{\partial^2 \theta}{\partial t^2} \ , \tag{S16}$$

where

$$\frac{dM_{\text{re}}}{dx} = \left( \sigma_{0,\text{A}} A_{\text{A}} \frac{\partial^2 v_{\text{A}}}{\partial x^2} - E_{\text{A}} I_{\text{A}} \frac{\partial^4 v_{\text{A}}}{\partial x^4} \right) d_{\text{A}} - \left( \sigma_{0,\text{B}} A_{\text{B}} \frac{\partial^2 v_{\text{B}}}{\partial x^2} - E_{\text{B}} I_{\text{B}} \frac{\partial^4 v_{\text{B}}}{\partial x^4} \right) d_{\text{B}} \ . \tag{S17}$$

The lever arms $d_{\text{A}}$ and $d_{\text{B}}$ can easily be calculated from the thickness of the two layers, $t_{\text{A}}$ and $t_{\text{B}}$, and the respective densities $\rho_{\text{A}}$ and $\rho_{\text{B}}$. For the parameter values given above we get $d_{\text{A}} = 84.1\,\text{nm}$ and $d_{\text{B}} = 15.9\,\text{nm}$. The polar moment of inertia is $I_{\text{p}} = 1.49 \cdot 10^{-28}\,\text{m}^4$ for the given beam cross-sectional area[S2]. For the shear modulus, we use the mean value $\mu = (\mu_{\text{A}} t_{\text{A}} + \mu_{\text{B}} t_{\text{B}})/(t_{\text{A}} + t_{\text{B}})$. With $\mu_{\text{Nb}} = 38\,\text{GPa}$[S10] and $\mu_{\text{SiN}} = 120\,\text{GPa}$[S11], we get $\mu = 91\,\text{GPa}$. The quantities $v_{\text{A}}$ and $v_{\text{B}}$ are related to the center-of-mass motion $v$ via $v_{\text{A}} = v - d_{\text{A}} \sin\theta$ and $v_{\text{B}} = v + d_{\text{B}} \sin\theta$ as one can see from Fig. S4(d). For small $\theta$, we can further approximate $\sin\theta \approx \theta$. For the following estimation, we assume $\theta(x,t) \propto v(x,t)$ with the proportionality constant $C = \theta/v$ and use the approximate beam displacement $v(x) \approx v_0 \cos(\pi x/L)$ (see Sec. B b). Substituting this into Eqs. (S16) and (S17) reveals that the equation of motion for the torsion [cf. Eq. (S16)] can be satisfied for all $x$ using the proportionality constant $C = 5.3 \cdot 10^4\,\text{rad/m}$. Thus, for a typical displacement of $v(0) = 1\,\text{nm}$, the corresponding twist angle is $\theta(0) = Cv(0) = 0.003°$.

### d. Torsion, elongation and bending energy

Finally, we calculate the torsional energy of the fundamental in-plane mode of the beam and compare it to the elongation and bending energy. The amount of energy stored in the torsion of the twisted beam is given by[S12]

$$U_{\text{torsion}} = \int_{-L/2}^{L/2} M_{\text{twist}}(x) \frac{d\theta}{dx} dx \ .$$

Using Eq. (S15), we find

$$U_{\text{torsion}} = \mu I_{\text{p}} \int_{-L/2}^{L/2} \left( \frac{d\theta}{dx} \right)^2 dx \ . \tag{S18}$$

The contribution of elongation and bending to the energy of a displaced nanomechanical beam have been derived by Unterreithmeier *et al.*[S7]. They are

$$U_{\text{elongation}} = \frac{A\sigma_{\text{eff}}}{2} \int_{-L/2}^{L/2} \left(\frac{\partial v}{\partial x}\right)^2 dx \tag{S19}$$

and

$$U_{\text{bending}} = \frac{w^3(t_{\text{A}} + t_{\text{B}})E_{\text{eff}}}{24} \int_{-L/2}^{L/2} \left(\frac{\partial^2 v}{\partial x^2}\right)^2 dx, \tag{S20}$$

where we have used the effective material parameters $\sigma_{\text{eff}}$ and $E_{\text{eff}}$ as justified above. Substituting $v(x) = v_0 \cos(\pi x/L)$ and $\theta(x) = Cv(x)$ into Eqs. (S18), (S19) and (S20), we find

$$U_{\text{torsion}} = 3.1 \cdot 10^{-21}\ \text{J}$$
$$U_{\text{elongation}} = 2.2 \cdot 10^{-19}\ \text{J}$$
$$U_{\text{bending}} = 6.4 \cdot 10^{-22}\ \text{J}$$

Hence, the torsional energy of the in-plane mode of the beam is about two orders of magnitude smaller than the total energy $U_{\text{tot}} = U_{\text{torsion}} + U_{\text{elongation}} + U_{\text{bending}}$. The torsional degree of freedom can therefore be neglected when describing the in-plane vibrational motion of the presented double-layer nanomechanical beam.

## ADDITIONAL REFERENCES


[S1] J. Weaver, W., S. P. Timoshenko, and D. H. Young, *Vibration Problems in Engineering* (John Wiley & Sons, 1990).

[S2] J. M. Gere and S. Timoshenko, *Mechanics of materials* (PWS-KENT Pub. Co., 1990).

[S3] W. Demtröder, *Experimentalphysik 1 - Mechanik und Wärme* (Springer, 2005).

[S4] A. N. Cleland, *Foundations of Nanomechanics* (Springer, 2003).

[S5] J. Rice, "Mechanics of solids," in *Encyclopaedia Britannica*, Vol. 23 (Encyclopaedia Britannica, Inc., 1993) pp. 732–747 and 773.

[S6] S. S. Verbridge, J. M. Parpia, R. B. Reichenbach, L. M. Bellan, and H. G. Craighead, "High quality factor resonance at room temperature with nanostrings under high tensile stress," Journal of Applied Physics **99**, 124304–124304–8 (2006).

[S7] Q. P. Unterreithmeier, T. Faust, and J. P. Kotthaus, "Damping of nanomechanical resonators," Physical Review Letters **105**, 027205 (2010).

[S8] We cannot directly access the compressive stress in our sputtered niobium films. The assumed stress, however, agrees with the stress measured for a similar sample and is consistent with values reported in literature for superconducting Nb thin films deposited by DC magnetron sputtering[S13].

[S9] M. Gad-el Hak, *The MEMS Handbook* (CRC Press, 2001).

[S10] This value was calculated from $\mu = E/(2(1+\nu))$[S4] with the Poisson ratio $\nu_{\mathrm{Nb}} = 0.40$[S4] and the Young's modulus $E_{\mathrm{Nb}} = 105\,\mathrm{GPa}$[S4].

[S11] M. Bauccio, ed., *ASM Engineered Materials Reference Book* (ASM International, 1994).

[S12] D. Kleppner and R. Kolenkow, *An introduction to mechanics* (McGraw-Hill, 1973).

[S13] T. Imamura, T. Shiota, and S. Hasuo, "Fabrication of high quality Nb/AlO/sub x/-Al/Nb josephson junctions. i. sputtered nb films for junction electrodes," IEEE Transactions on Applied Superconductivity **2**, 1–14 (1992).
